# Supplementary material for: Strain- and Field-Tunable Nonrelativistic Spin Splitting and Wave-Symmetry-Dependent Spin Transport in Twisted Bilayer Altermagnets
Source: arXiv:2602.19713 source file (2026-02-23)
Supplement: Supplementary file 1 [file SI.pdf]

# Supporting Information for “Strain- and Field-Tunable Nonrelativistic Spin Splitting and Wave-Symmetry–Dependent Spin Transport in Twisted Bilayer Altermagnets”

Shantanu Pathak\* and Saswata Bhattacharya\*

*Department of Physics, Indian Institute of Technology Delhi, New Delhi 110016, India*

E-mail: shantanu.pathak@physics.iitd.ac.in; saswata@physics.iitd.ac.in

This Supporting Information includes:

- Charge conductivity  $\sigma_{xx}^z$  and  $\sigma_{yy}^z$  as a function of energy for (a) twisted bilayer  $\text{CoCl}_2$  and (b) twisted bilayer  $\text{MnTe}_2$ .
- Linear nonrelativistic spin-splitting coefficient  $\alpha^{(1)}$  (meV Å) as a function of biaxial strain for representative twisted bilayers.
- Electric-field-induced spin splitting  $\Delta$  at the VBM and CBM as a function of out-of-plane electric field  $\mathcal{E}_z$  for representative hexagonal and tetragonal twisted bilayers.

1 Charge conductivity  $\sigma_{xx}^z$  and  $\sigma_{yy}^z$  as a function of energy for (a) twisted bilayer  $\text{CoCl}_2$  and (b) twisted bilayer  $\text{MnTe}_2$ .

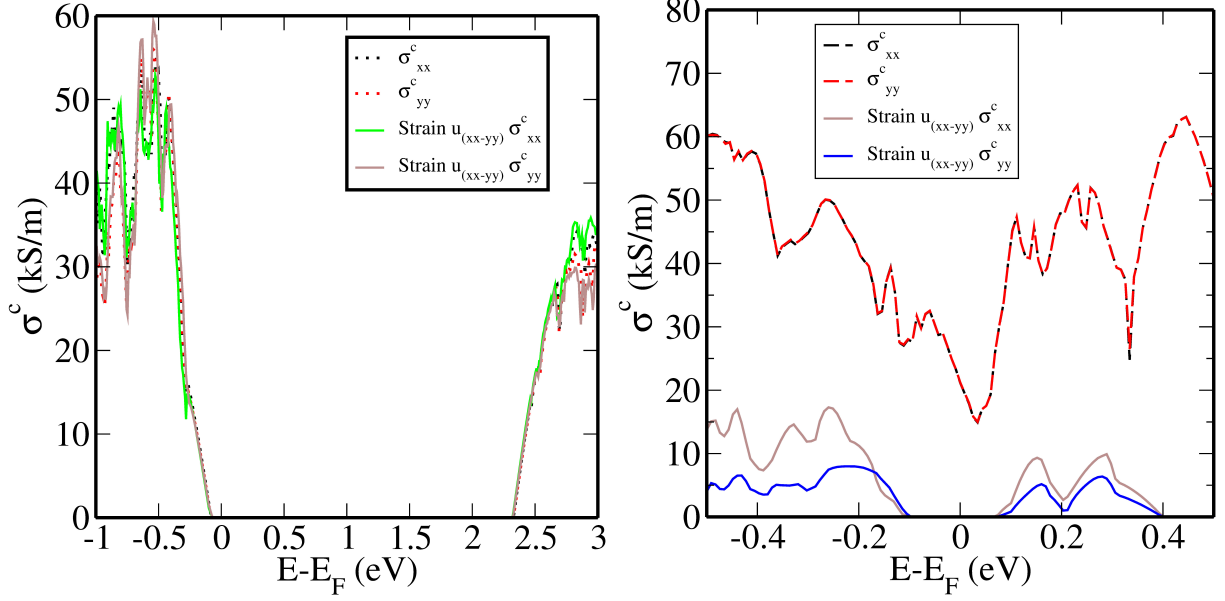

Figure 1: Charge conductivity  $\sigma_{xx}^z$  and  $\sigma_{yy}^z$  as a function of energy for (a) twisted bilayer  $\text{CoCl}_2$  and (b) twisted bilayer  $\text{MnTe}_2$ , shown for unstrained and strained configurations. Strain modifies the energy dependence and anisotropy of the charge transport response.

## 2 Linear nonrelativistic spin-splitting coefficient $\alpha^{(1)}$ (meV Å) as a function of biaxial strain for representative twisted bilayers.

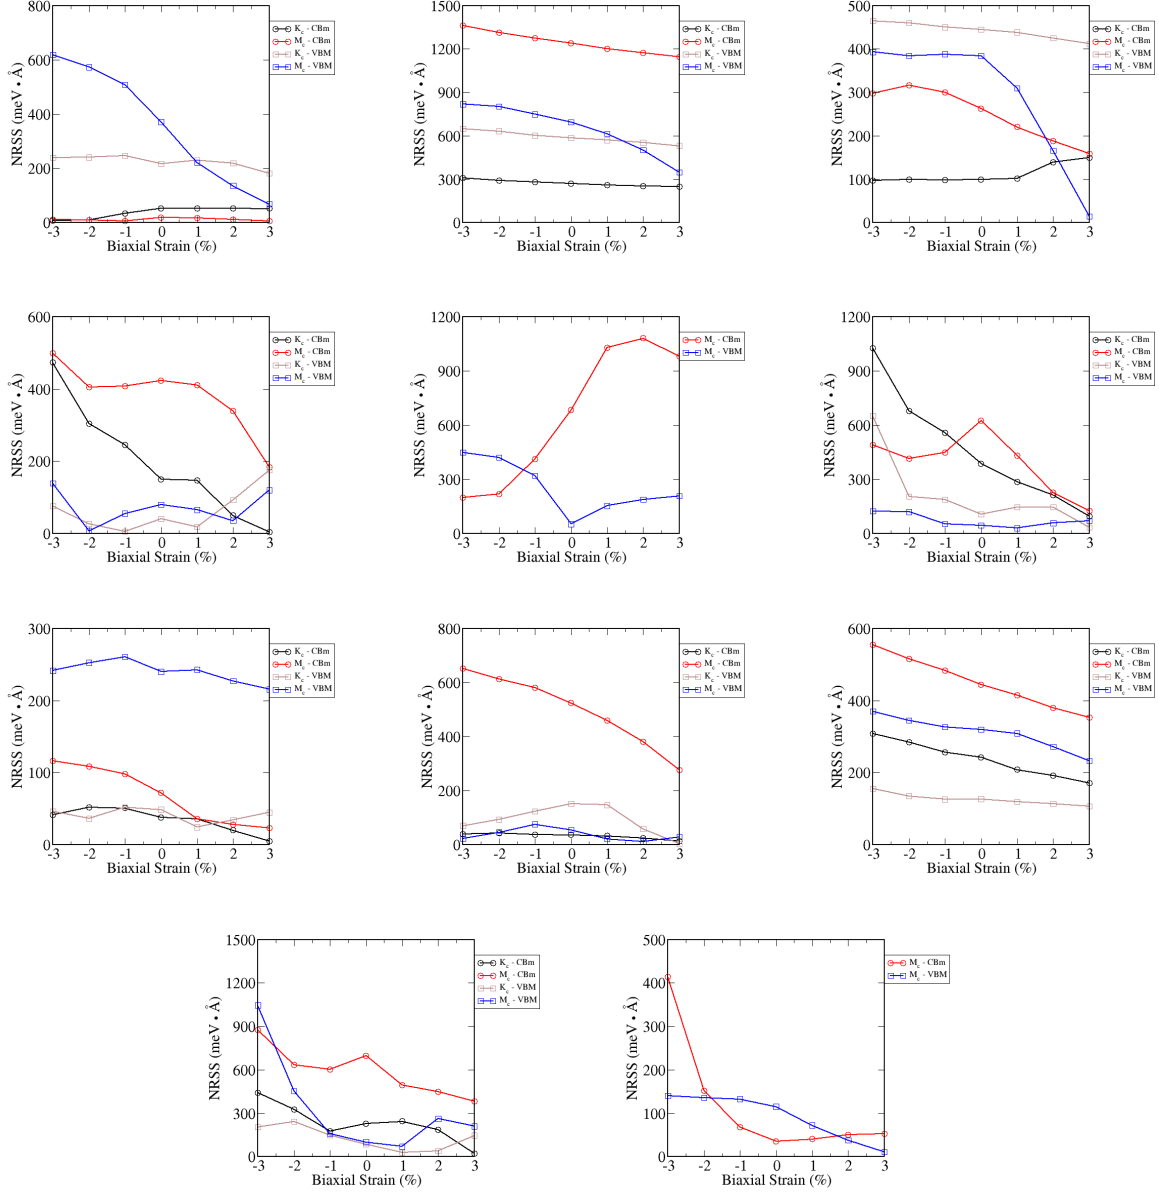

**Figure S2.** Linear nonrelativistic spin-splitting coefficient  $\alpha^{(1)}$  (meV Å) as a function of biaxial strain for twisted bilayer (a)  $\text{CoCl}_2$  (hexa), (b)  $\text{MnI}_2$ , (c)  $\text{NiBr}_2$ , (d)  $\text{VCl}_2$ , (e)  $\text{CoS}$ , (f)  $\text{MnSe}_2$ , (g)  $\text{NiF}_2$ , (h)  $\text{VI}_2$ , (i)  $\text{MnCl}_2$ , (j)  $\text{MnTe}_2$ , and (k)  $\text{RuSe}$ . Biaxial strain modifies the magnitude of NRSS while preserving the underlying spin-wave symmetry.

### 3 Electric-field-induced spin splitting for representative hexagonal and tetragonal twisted bilayers

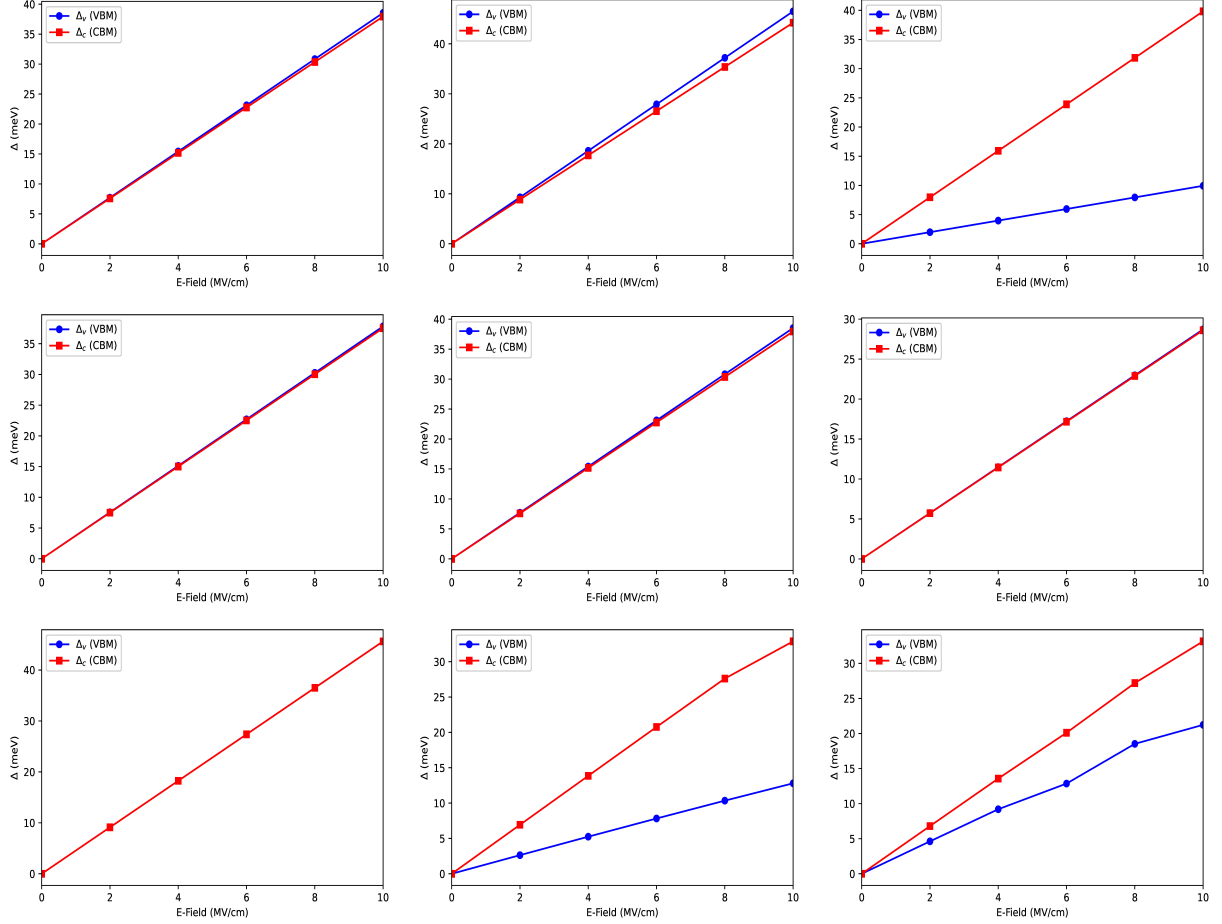

**Figure S3.** Electric-field-induced spin splitting  $\Delta$  at the VBM and CBM as a function of out-of-plane electric field  $\mathcal{E}_z$  for representative twisted bilayers. Hexagonal systems: (a)  $\text{CoCl}_2$ , (b)  $\text{MnI}_2$ , (c)  $\text{MnSe}_2$ , (d)  $\text{VCl}_2$ , (e)  $\text{MnCl}_2$ , (f)  $\text{NiF}_2$ , and (g)  $\text{VI}_2$ . Tetragonal systems: (h)  $\text{RuSe}$  and (i)  $\text{CoS}$ . In all cases,  $\Delta$  exhibits an approximately linear dependence on  $\mathcal{E}_z$ , consistent with field-induced symmetry breaking.
